# Supplementary material for: LEMMo-Plan: LLM-Enhanced Learning from Multi-Modal Demonstration for Planning Sequential Contact-Rich Manipulation Tasks
Source: arXiv:2409.11863 source file (2025-03-10)
Supplement: Supplementary file 1 [file Appendix.tex]

\appendix
\section{Visual-Tactile Segmentation with LLMs}~\label{sec: appendix}

\section{Extraction of Example Task Plan from Demonstration}
\subsection{PDDL domain generated from skill library}~\label{apd: initial_domain}
\begin{lstlisting}
{
    "role": "system", 
    "content":"You are reasoning about robot skills and skill parameters at each frame of a video step by step. Skill has to be selected from the following skill library."
},
{
    "role": "user",
    "content": "Your reasoning will be based on PDDL. Before reasoning, generate a PDDL domain of the skill library: " + prompt_skill_library + "Format your answer strictly in the way: (define (domain robot_skills)"           
}
\end{lstlisting}
\begin{lstlisting}
(define (domain robot_skills)
  (:requirements :strips :typing)
  (:types pose direction object)

  (:predicates
    (at ?p - pose)
    (holding_cable_head)
    (hand_open)
    (cable_stretched)
    (cable_inserted ?d - direction ?o - object)
  )

  (:action move
    :parameters (?p - pose)
    :precondition (and (hand_open))
    :effect (and (at ?p))
  )

  (:action move_cable_head
    :parameters (?p - pose)
    :precondition (and (holding_cable_head))
    :effect (and (at ?p))
  )

  (:action grasp
    :parameters ()
    :precondition (and (hand_open))
    :effect (and (holding_cable_head) (not (hand_open)))
  )

  (:action open_hand
    :parameters ()
    :precondition (and (holding_cable_head))
    :effect (and (hand_open) (not (holding_cable_head)))
  )

  (:action stretch
    :parameters ()
    :precondition (and (holding_cable_head))
    :effect (and (cable_stretched))
  )

  (:action insert
    :parameters (?d - direction ?o - object)
    :precondition (and (holding_cable_head) (at ?p))
    :effect (and (cable_inserted ?d ?o) (not (holding_cable_head)) (hand_open))
  )
)

\end{lstlisting}

\begin{lstlisting}
promt_task_description = ''' 
The video is about two robot hands mounting a cable onto several clips. Each frame has been annotated with the status of the cable collected by the tactile sensor, and the clip positions (red bounding box) and openning directions (yellow arrow). The blue curve in the view is the cable.
'''

pddl_prompt_example = '''
Frame 1 (19:35:27.208): (move clip2) ; Because one of the robot is moving with cable grasped to the position of clip 2
'''.strip()

{
    "role": "user",
    "content": 
    ["As the first step of your reasoning, reason which skill in the skill library (defined already as PDDL domain) the robot performs at each frame. ",
     "Below are key frames from the video to be described.", 
    promt_task_description,
    *map(lambda x: {"type": "image_url", "image_url": {"url": f'data:image/jpg;base64,{x}', "detail": "high"}}, visual_tactile_processed),
    "Format your reasoning as strings strictly in 'frame number(timestamp): skill and reason' format. For example, " + pddl_prompt_example,
    "Consider the annotated obejct status and also the robot movement in video frames in your reasoning."
    ]
},
\end{lstlisting}

\begin{lstlisting}
Frame 1 (19:22:34.591): (move_object cable clip1) ; Because the robot is moving with the cable towards the position of clip1 and the tactile status is idle.

Frame 2 (19:22:39.539): (grasp cable) ; Because the tactile status indicates that the cable is grasped.

Frame 3 (19:22:45.095): (stretch cable) ; Because the tactile status indicates the cable is under linear force, suggesting the robot is stretching the cable.

Frame 4 (19:22:46.902): (stretch cable) ; Because the tactile status indicates the cable is still under linear force, suggesting the robot is continuing to stretch the cable.

Frame 5 (19:22:52.891): (insert cable downward clip1) ; Because the tactile status indicates the cable is under torque, suggesting the robot is inserting the cable into clip1 in the downward direction.

Frame 6 (19:22:57.987): (insert cable downward clip1) ; Because the tactile status indicates the cable is still under torque, suggesting the robot is continuing to insert the cable into clip1 in the downward direction.

Frame 7 (19:23:01.407): (insert cable downward clip1) ; Because the tactile status indicates the torque has stopped, suggesting the robot has finished inserting the cable into clip1 in the downward direction.

Frame 8 (19:23:05.705): (open_hand) ; Because the tactile status indicates the cable is released, suggesting the robot has opened its hand to release the cable.

\end{lstlisting}

\textbf{Skill Reasoning Without Object Status}
\begin{lstlisting}
Frame 1 (19:22:34.591): (move_cable_head clip1) ; Because the robot is holding the cable head and moving towards the position of clip 1.

Frame 2 (19:22:39.539): (move_cable_head clip1) ; Because the robot is still holding the cable head and continuing to move towards the position of clip 1.

Frame 3 (19:22:45.005): (move_cable_head clip1) ; Because the robot is holding the cable head and is almost at the position of clip 1.

Frame 4 (19:22:46.902): (move_cable_head clip1) ; Because the robot is holding the cable head and is very close to the position of clip 1.

Frame 5 (19:22:52.891): (insert downward clip1) ; Because the robot is holding the cable head and is in position to insert the cable into clip 1 in the downward direction.

Frame 6 (19:22:57.987): (insert downward clip1) ; Because the robot is holding the cable head and is in the process of inserting the cable into clip 1 in the downward direction.

Frame 7 (19:23:01.407): (insert downward clip1) ; Because the robot is holding the cable head and is still in the process of inserting the cable into clip 1 in the downward direction.

Frame 8 (19:23:05.705): (insert downward clip1) ; Because the robot is holding the cable head and is completing the insertion of the cable into clip 1 in the downward direction.

\end{lstlisting}
